# Supplementary material for: Memorization to Generalization: Emergence of Diffusion Models from Associative Memory
Source: arXiv:2505.21777 source file (2026-03-16)
Supplement: Supplementary file 16 [file relative_energy_interp.tex]

\begin{figure}[!t]
\centering
\includegraphics[keepaspectratio, width=0.9\textwidth, height=1.0\textheight]{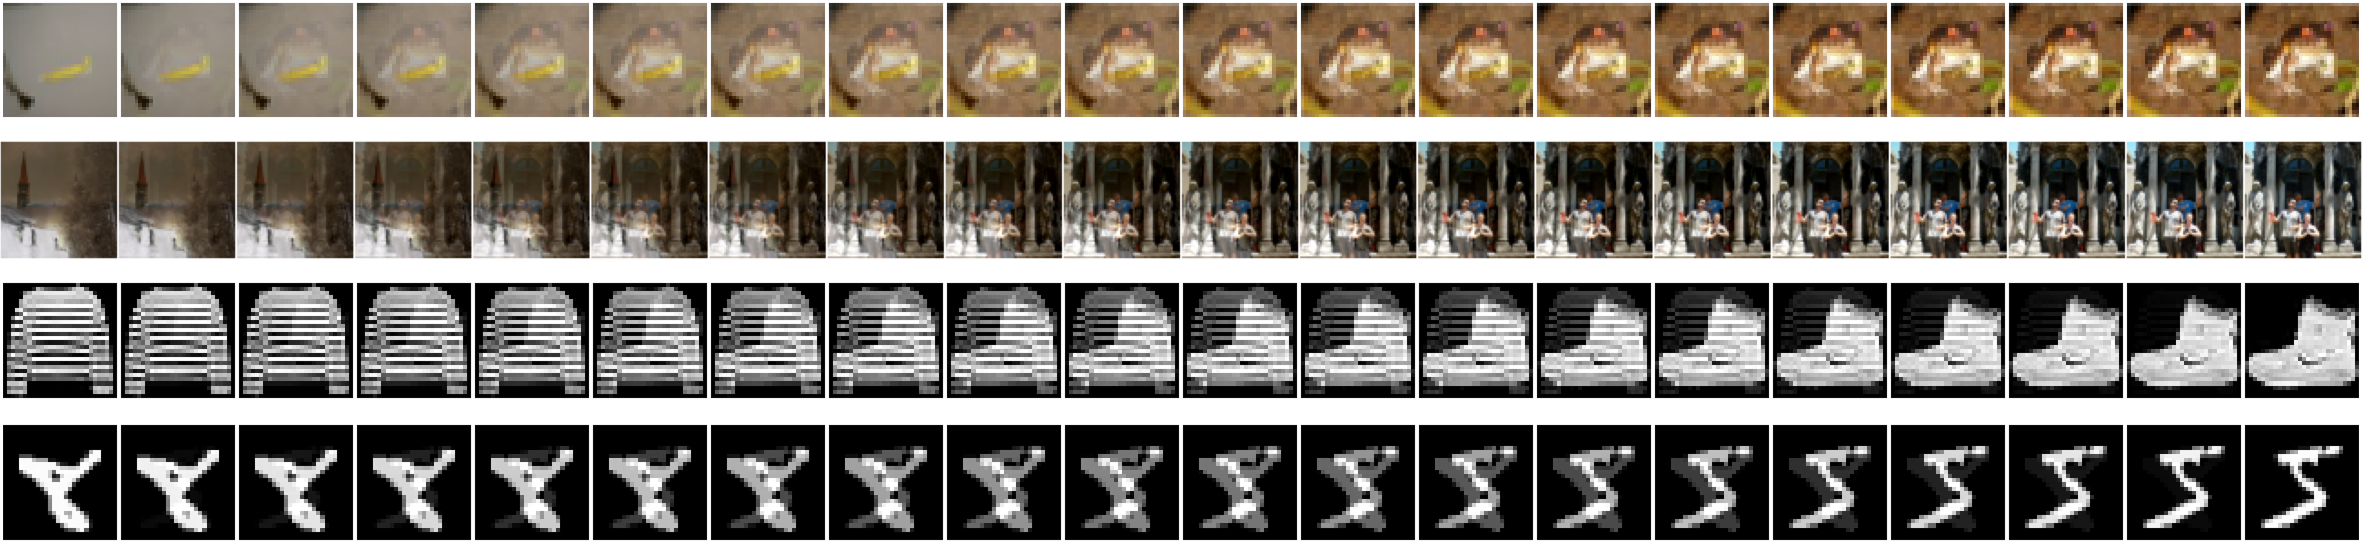}

\internallinenumbers

\caption{Circular interpolation of a target image $\rvx_1$ and a reference image $\rvx_2$ over $\alpha \in \{0, \dots, \frac{\pi}{2}\}$ for different datasets.}

\label{fig:relative-energy-interpolation}

\end{figure}
