# Supplementary material for: Memorization to Generalization: Emergence of Diffusion Models from Associative Memory
Source: arXiv:2505.21777 source file (2026-03-16)
Supplement: Supplementary file 21 [file critical_time_alg.tex]

\begin{algorithm}[H]
\caption{Compute critical time $t_c$ for a pattern}
\label{alg:critical_time}

\DontPrintSemicolon

\SetKwProg{initialize}{Initialize}{}{end}
\SetKwProg{inputs}{Inputs}{}{end}
\SetKwProg{output}{Output}{}{end}
\SetKwProg{params}{Parameters}{}{end}
\SetKwProg{hyperparams}{HyperParameters}{}{end}
\SetKwProg{train}{Train}{}{end}
\SetKwProg{infer}{Compute $t_c$}{}{end}
\SetArgSty{textnormal}
\SetKwInOut{Input}{Input}
\SetKwInOut{Output}{Output}

\inputs{}{\vspace{1.5pt}
Pattern $\hat{\rvx}$\; \vspace{1.5pt}
Time stride $s$\; \vspace{1.5pt}
Score model $s_\theta$\; \vspace{1.5pt}
DDIM sampler $\Phi$\; \vspace{1.5pt}
Error threshold $\delta_d$\; \vspace{1.5pt}
Distance metric $d$\;  \vspace{1.5pt}
Denoising steps $N'$\; \vspace{1.5pt}
Total diffusion time $T$\;  \vspace{1.5pt}
Number of trials $M$\; \vspace{1.5pt}
Probability threshold $\delta_p$\; \vspace{1.5pt}
Forward process $\mathcal{F}$ 
}
\infer{}{%
\vspace{5pt}
$\rvx_0 \gets \text{duplicate}(\hat{\rvx}, M)$ \tcp*{\small Duplicate pattern for $M$ times} \vspace{5pt} 
$t_c \gets \mathbf{0}$ \tcp*{\small Initialize critical time tracker} \vspace{5pt}
$\hat{S} \gets \mathbf{0}$ \tcp*{\small Track trials that have stopped} \vspace{5pt} 
\For{$t = 1, 1+s, 1+2s, \dots, T - s - 1$}{\vspace{5pt}
    $\epsilon \sim \mathcal{N}(0, I)$ \tcp*{\small Sample noise} \vspace{5pt} 
    
    $\rvx_t \gets \mathcal{F}(\rvx_0, \epsilon, t)$ \tcp*{\small Forward process} \vspace{5pt} 
    
    $\hat{\rvx}_0 \gets \Phi(s_\theta, \rvx_t, t, N')$ \tcp*{\small DDIM denoising} \vspace{5pt} 
    
    $\mathbf{d} \gets d(\hat{\rvx}_0, \rvx_0)$ \tcp*{\small Compute distance per trial} \vspace{8pt} 
    
    $\mathbf{r}_i \gets 
        \begin{cases}
            1 & \text{if } \mathbf{d}_i \leq \delta_d \\
            0 & \text{otherwise}
        \end{cases}$ for $i = 1, \dots, M$ \tcp*{\small Binary recovery vector} \vspace{8pt} 
    
    $p \gets \frac{1}{M} \sum_{i=1}^M \mathbf{r}_i$ \tcp*{\small Recovery probability} \vspace{8pt} 
    
    \eIf{$p < \delta_p$}{
        \Return $t_c$ 
    }{
        $\hat{S} \gets \text{update}(\hat{S}, \mathbf{r})$ \;
        $t_c \gets \text{update}(t, t_c, \hat{S})$ 
    }
}
}
\output{}{\vspace{5pt}
Critical time $t_c \in \mathbb{N}^M$}
\end{algorithm}
